# Supplementary material for: Double excitations in molecules
Source: arXiv:2508.16262 source file (2025-09-01)
Supplement: Supplementary file 1 [file Supplementary_Material.pdf]

# Supplementary Material for "Double excitations in molecule"

## I Total spin $S^2$ eigenstates

We constructed (total) spin eigenstates for each type of Slater determinant (SD) separately. The spin eigenstates are denoted as $|X_n^m\rangle$, where X corresponds to $S^2$ eigenvalue (S for singlet, T for triplet and Q for quintet),$m$ corresponds to eigenvalue of $S_z$ and $n$ corresponds to the index of a state with a given $S^2$ and $S_z$ eigenvalue.

For singly excited SDs, the spin eigenstates consist of one singlet and three triplet states (each corresponding to $S_z = -1, 0, 1$).

$$\left|S_1^0\right\rangle = \frac{1}{\sqrt{2}}[|\uparrow\uparrow\rangle + |\downarrow\downarrow\rangle]$$
$$\left|T_1^{-1}\right\rangle = |\downarrow\uparrow\rangle$$
$$\left|T_1^{+1}\right\rangle = \frac{1}{\sqrt{2}}[|\uparrow\uparrow\rangle - |\downarrow\downarrow\rangle]$$
$$\left|T_1^0\right\rangle = |\uparrow\downarrow\rangle$$

For group I doubly excited SDs the spin eigenstates contain five quintet states (each corresponding to $S_z$ = -2,-1,0,1,2), nine triplet states, and two singlet states. We give below the spin structures of these spin eigenstates, which are essentially the same as those given by Scholes[1]. However, while Scholes used particle creation operators acting on the vacuum state to construct the SDs, we have employed electron-hole creation operators acting on the non-interacting ground state to construct the SDs.

$$\left|S_2^0\right\rangle = \frac{1}{\sqrt{3}}(|\uparrow\uparrow\uparrow\uparrow\rangle + |\downarrow\downarrow\downarrow\downarrow\rangle$$
$$+ \frac{1}{2}(|\uparrow\downarrow\uparrow\downarrow\rangle + |\downarrow\uparrow\downarrow\uparrow\rangle + |\uparrow\downarrow\downarrow\uparrow\rangle + |\downarrow\uparrow\uparrow\downarrow\rangle)))$$
$$\left|S_3^0\right\rangle = \frac{1}{2}(|\uparrow\downarrow\uparrow\downarrow\rangle + |\downarrow\uparrow\downarrow\uparrow\rangle - |\uparrow\downarrow\downarrow\uparrow\rangle - |\downarrow\uparrow\uparrow\downarrow\rangle)$$
$$\left|T_4^0\right\rangle = \frac{1}{\sqrt{3}}(|\uparrow\uparrow\uparrow\uparrow\rangle - |\downarrow\downarrow\downarrow\downarrow\rangle$$
$$- \frac{1}{2}(|\uparrow\downarrow\uparrow\downarrow\rangle + |\downarrow\uparrow\downarrow\uparrow\rangle - |\uparrow\downarrow\downarrow\uparrow\rangle - |\downarrow\uparrow\uparrow\downarrow\rangle))$$
$$\left|T_5^0\right\rangle = \frac{1}{\sqrt{6}}(|\uparrow\uparrow\uparrow\uparrow\rangle - |\downarrow\downarrow\downarrow\downarrow\rangle$$
$$+ |\uparrow\downarrow\uparrow\downarrow\rangle + |\downarrow\uparrow\uparrow\downarrow\rangle - |\downarrow\uparrow\downarrow\uparrow\rangle - |\uparrow\downarrow\downarrow\uparrow\rangle)$$
$$\left|T_6^0\right\rangle = \frac{1}{2}(|\uparrow\downarrow\uparrow\downarrow\rangle + |\uparrow\downarrow\downarrow\uparrow\rangle - |\downarrow\uparrow\uparrow\downarrow\rangle - |\downarrow\uparrow\downarrow\uparrow\rangle)$$
$$\left|T_4^{+1}\right\rangle = \frac{1}{\sqrt{6}}(2\,|\uparrow\uparrow\uparrow\downarrow\rangle + |\uparrow\downarrow\downarrow\downarrow\rangle + |\downarrow\uparrow\downarrow\downarrow\rangle)$$
$$\left|T_5^{+1}\right\rangle = \frac{1}{2\sqrt{3}}(3\,|\uparrow\uparrow\downarrow\uparrow\rangle + |\uparrow\downarrow\downarrow\downarrow\rangle + |\downarrow\uparrow\downarrow\downarrow\rangle - |\uparrow\uparrow\uparrow\downarrow\rangle)$$
$$\left|T_6^{+1}\right\rangle = \frac{1}{\sqrt{2}}(\uparrow\downarrow\downarrow\downarrow - \downarrow\uparrow\downarrow\downarrow)$$
$$\left|T_4^{-1}\right\rangle = \frac{1}{\sqrt{6}}(2\,|\downarrow\downarrow\downarrow\uparrow\rangle\,|\uparrow\downarrow\uparrow\uparrow\rangle + |\downarrow\uparrow\uparrow\uparrow\rangle)$$
$$\left|T_5^{-1}\right\rangle = \frac{1}{2\sqrt{3}}(3\,|\downarrow\downarrow\uparrow\downarrow\rangle + |\downarrow\uparrow\uparrow\uparrow\rangle + |\downarrow\uparrow\uparrow\uparrow\rangle - |\downarrow\downarrow\downarrow\uparrow\rangle)$$
$$\left|T_6^{-1}\right\rangle = \frac{1}{\sqrt{2}}(|\uparrow\downarrow\uparrow\uparrow\rangle - |\downarrow\uparrow\uparrow\uparrow\rangle)$$
$$\left|Q_1^{+2}\right\rangle = |\uparrow\uparrow\downarrow\downarrow\rangle$$
$$\left|Q_1^{+1}\right\rangle = \frac{1}{2}(|\uparrow\downarrow\uparrow\uparrow\rangle + |\downarrow\uparrow\uparrow\uparrow\rangle - |\uparrow\uparrow\uparrow\downarrow\rangle - |\uparrow\uparrow\downarrow\uparrow\rangle)$$
$$\left|Q_1^0\right\rangle = \frac{1}{\sqrt{6}}(|\uparrow\uparrow\uparrow\uparrow\rangle + |\downarrow\downarrow\downarrow\downarrow\rangle$$
$$- |\uparrow\downarrow\uparrow\downarrow\rangle - |\downarrow\uparrow\downarrow\uparrow\rangle - |\uparrow\downarrow\downarrow\uparrow\rangle - |\downarrow\uparrow\uparrow\downarrow\rangle)$$
$$\left|Q_1^{-1}\right\rangle = \frac{1}{2}(|\uparrow\downarrow\downarrow\downarrow\rangle + |\downarrow\uparrow\downarrow\downarrow\rangle - |\uparrow\uparrow\uparrow\downarrow\rangle - |\uparrow\uparrow\downarrow\uparrow\rangle)$$
$$\left|Q_1^{-2}\right\rangle = |\downarrow\downarrow\uparrow\uparrow\rangle$$

For group II double excited SDs the spin eigenstates contain one singlet and three triplet states.

$$\left|S_4^0\right\rangle = \frac{1}{\sqrt{2}}(|\uparrow\downarrow\uparrow\downarrow\rangle - |\downarrow\uparrow\uparrow\downarrow\rangle)$$
$$\left|T_7^{+1}\right\rangle = |\uparrow\uparrow\uparrow\downarrow\rangle$$
$$\left|T_7^0\right\rangle = \frac{1}{\sqrt{2}}(|\uparrow\downarrow\uparrow\downarrow\rangle + |\downarrow\uparrow\uparrow\downarrow\rangle)$$
$$\left|T_7^{-1}\right\rangle = |\downarrow\downarrow\uparrow\downarrow\rangle$$

Similarly, for group III doubly excited SDs, the spin eigenstates consist of one singlet and three triplet states.

$$\left|S_5^0\right\rangle = \frac{1}{\sqrt{2}}(|\uparrow\downarrow\uparrow\downarrow\rangle - |\uparrow\downarrow\downarrow\uparrow\rangle)$$
$$\left|T_8^{+1}\right\rangle = |\uparrow\downarrow\downarrow\downarrow\rangle$$
$$\left|T_8^0\right\rangle = \frac{1}{\sqrt{2}}(|\uparrow\downarrow\uparrow\downarrow\rangle + |\uparrow\downarrow\downarrow\uparrow\rangle)$$
$$\left|T_8^{-1}\right\rangle = |\uparrow\downarrow\uparrow\uparrow\rangle$$

The group IV doubly excited SDs can only form a singlet state.

$$\left|S_6^0\right\rangle = |\uparrow\downarrow\uparrow\downarrow\rangle$$

## II Thiel's set results

| | Molecule | Symmetry | Best Theoretical Estimate[2] | GW-BSE (full)[3] | GW-BSE (TDA) | scrCISD | scrCIS(D) |
|---|---|---|---|---|---|---|---|
| Series 1 | Ethene | $B_{1u}$ | 7.8 | 7.7 | 8.47 | 7.42 | 8.42 |
| | E-Butadiene | $B_u$ | 6.18 | 5.88 | 6.49 | 5.63 | 6.32 |
| | | $A_g$ | 6.55 | 7.45 | 7.47 | 5.89 | 6.99 |
| | all-E-Hexatriene | $B_u$ | 5.10 | 4.87 | 5.39 | 4.53 | 5.19 |
| | | $A_g$ | 5.09 | 6.49 | 6.50 | 4.80 | 5.94 |
| | all-E-Octatetraene | $A_g$ | 4.47 | 5.71 | 5.73 | - | 5.16 |
| | | $B_u$ | 4.66 | 4.23 | 4.68 | - | 4.47 |
| | Cyclopropene | $B_1$ | 6.76 | 6.66 | 6.68 | 5.68 | 6.53 |
| | | $B_2$ | 7.06 | 6.65 | 7.09 | 6.16 | 6.98 |
| | Cyclopentadiene | $B_1$ | 5.55 | 5.07 | 5.53 | 4.73 | 5.41 |
| | | $A_1$ | 6.31 | 6.83 | 6.83 | 5.64 | 6.58 |
| | Norbornadiene | $A_2$ | 5.34 | 5.19 | 5.47 | - | 5.21 |
| | | $B_2$ | 6.11 | 6.23 | 6.31 | - | 5.92 |
| Series 2 | Benzene | $B_{2u}$ | 5.08 | 5.21 | 5.24 | - | 5.01 |
| | | $B_{1u}$ | 6.54 | 6.05 | 6.31 | - | 6.29 |
| | | $E_{1u}$ | 7.13 | 6.92 | 7.58 | - | 7.05 |
| | | $E_{1g}$ | 8.41 | 8.83 | 8.92 | - | 8.68 |
| | Naphthalene | $A_g$ | 5.87 | 6.12 | 7.19 | - | 6.75 |
| | | $A_g$ | 6.67 | 7.24 | 7.24 | - | 7.00 |
| | | $B_{1g}$ | 5.99 | 5.91 | 5.92 | - | 5.45 |
| | | $B_1g$ | 6.47 | 6.26 | 6.6 | - | 6.48 |
| | | $B_{2u}$ | 4.77 | 4.42 | 4.67 | - | 4.5 |
| | | $B_{2u}$ | 6.33 | 6.09 | 6.46 | - | 6.29 |
| | | $B_{3u}$ | 4.24 | 4.33 | 4.36 | - | 4.12 |
| | | $B_{3u}$ | 6.06 | 5.83 | 6.37 | - | 5.92 |
| | Furan | $B_2$ | 6.32 | 6.17 | 6.62 | 5.75 | 6.56 |
| | | $A_1$ | 6.57 | 6.77 | 6.83 | 5.56 | 6.47 |
| | Pyrrole | $A_1$ | 6.37 | 6.76 | 6.76 | 5.85 | 6.51 |
| | | $B_2$ | 6.57 | 6.37 | 6. 77 | 5.86 | 6.28 |
| | Imidazole | $A'$ | 6.19 | 6.45 | 6.72 | 5.50 | 6.51 |
| | | $A'$ | 6.93 | 6.97 | 7.18 | 5.60 | 7.18 |
| | | $A''$ | 6.81 | 6.59 | 6.62 | 5.48 | 6.27 |
| | Pyridine | $B_1$ | 4.59 | 4.95 | 5.02 | - | 4.73 |
| | | $B_2$ | 4.85 | 5.27 | 5.35 | - | 5.12 |
| | | $A_2$ | 5.11 | 5.29 | 5.29 | - | 4.86 |
| | Pyrimidine | $B_2$ | 5.44 | 5.48 | 5.56 | - | 5.30 |
| | | $A_2$ | 4.91 | 4.72 | 4.74 | - | 4.32 |
| | Pyrazine | $A_u$ | 4.81 | 4.86 | 4.87 | - | 4.43 |
| | | $B_{2u}$ | 4.64 | 5.10 | 5.25 | - | 5.06 |
| | | $B_{3u}$ | 3.95 | 4.08 | 4.16 | - | 3.94 |
| | Pyridazine | $A_1$ | 5.18 | 5.34 | 5.43 | - | 5.17 |
| | | $A_2$ | 4.32 | 4.34 | 4.37 | - | 3.95 |
| | | $B_1$ | 3.78 | 3.70 | 3.80 | - | 3.54 |
| | s-Triazine | $A'_2$ | 5.79 | 5.83 | 5.86 | - | 5.62 |
| | | $A''_1$ | 4.6 | 4.54 | 4.54 | - | 4.12 |
| | | $A''_2$ | 4.66 | 4.68 | 4.74 | - | 4.43 |
| | | $E''$ | 4.7 | 4.64 | 4.67 | - | 4.39 |
| | s-Tetrazine | $A_u$ | 3.51 | 3.64 | 3.67 | - | 3.25 |
| | | $A_u$ | 5.5 | 5.34 | 5.39 | - | 5.18 |
| | | $B_{1g}$ | 4.73 | 4.83 | 4.95 | - | 4.55 |
| | | $B_{2g}$ | 5.2 | 5.34 | 5.38 | - | 5.18 |
| | | $B_{3u}$ | 4.93 | 5.2 | 5.39 | - | 5.16 |
| | | $B_{2u}$ | 2.29 | 2.26 | 2.37 | - | 2.15 |
| Series 3 | Formaldehyde | $A_2$ | 3.88 | 3.77 | 3.81 | 2.75 | 3.66 |
| | | $B_1$ | 9.10 | 8.84 | 8.92 | 7.84 | 8.74 |
| | | $A1$ | 9.30 | 9.70 | 9.71 | 8.75 | 9.45 |
| | Formamide | $A''$ | 5.63 | 5.36 | 5.37 | 4.72 | 5.12 |
| | | $A'$ | 7.39 | 8.18 | 8.36 | 7.11 | 7.79 |
| | Acetone | $A_2$ | 4.4 | 4.19 | 4.22 | - | 3.98 |

| | | | | | | | |
|---|---|---|---|---|---|---|---|
| | | $A_1$ | 9.4 | 9.47 | 9.88 | - | 9.66 |
| | | $B_1$ | 9.1 | 9.2 | 9.28 | - | 8.9 |
| | p-Benzoquinone | $A_u$ | 2.77 | 2.77 | 2.8 | - | 2.42 |
| | | $B_{1g}$ | 2.76 | 2.72 | 2.75 | - | 2.42 |
| | | $B_{1u}$ | 5.28 | 5.06 | 5.54 | - | 5.2 |
| | | $B_{2g}$ | 4.26 | 4.25 | 4.53 | - | 3.89 |
| | | $B_{2u}$ | 6.96 | 7.07 | 7.07 | - | 6.39 |
| | | $B_{3u}$ | 5.64 | 5.95 | 5.97 | - | 5.55 |
| | Acetamide | $A''$ | 5.69 | 5.39 | 5.40 | 4.24 | 5.12 |
| | | $A'$ | 7.27 | 7.56 | 7.83 | 6.50 | 7.34 |
| | Propanamide | $A''$ | 5.72 | 5.41 | 5.43 | 4.53 | 5.13 |
| | | $A'$ | 7.20 | 7.56 | 7.78 | 6.60 | 7.19 |
| Series 4 | Cytosine | $A'$ | 4.66 | 4.59 | 4.81 | - | 4.37 |
| | | $A'$ | 5.62 | 5.55 | 5.75 | - | 5.33 |
| | | $A''$ | 4.87 | 4.96 | 4.98 | - | 4.5 |
| | | $A''$ | 5.26 | 5.59 | 5.6 | - | 5.59 |
| | Thymine | $A'$ | 5.2 | 5.13 | 5.44 | - | 5.03 |
| | | $A'$ | 6.27 | 6.26 | 6.45 | - | 5.97 |
| | | $A'$ | 6.53 | 6.69 | 6.87 | - | 6.38 |
| | | $A''$ | 4.82 | 4.74 | 4.76 | - | 4.37 |
| | | $A''$ | 6.16 | 6.08 | 6.09 | - | 5.67 |
| | Uracil | $A'$ | 5.35 | 5.24 | 5.55 | - | 5.14 |
| | | $A'$ | 6.26 | 6.21 | 6.37 | - | 5.99 |
| | | $A'$ | 6.7 | 6.82 | 6.99 | - | 6.51 |
| | | $A''$ | 4.8 | 4.7 | 4.72 | - | 4.26 |
| | | $A''$ | 6.1 | 6.01 | 5.58 | - | 5.58 |
| | | $A''$ | 6.56 | 6.71 | 6.71 | - | 6.25 |
| | Adenine | $A'$ | 5.25 | 5.18 | 5.2 | - | 4.75 |
| | | $A'$ | 5.25 | 5.18 | 5.23 | - | 4.89 |
| | | $A''$ | 5.12 | 5.1 | 5.37 | - | 5.05 |
| | | $A''$ | 5.75 | 5.79 | 5.82 | - | 5.49 |
| | MSE | | ... | 0.05 | 0.20 | -0.81 | -0.12 |
| | MAE | | ... | 0.22 | 0.28 | 0.81 | 0.29 |

# III The multichannel Dyson equation

The multichannel Dyson equation[4–6] (MCDE), couples two or more $n$-body (time-ordered) Green's functions. We specifically focus on the MCDE that couples the 2-body Green's function with the 4-body Green's function. Let $G_4^0$ be a non-interacting four-body Green's function. Under the time constraint that enforces the simultaneous creation of two electrons and two holes and their simultaneous destruction, the number of free time variables reduces from eight to two. Taking the Fourier transform with respect to the time difference of the two free time variables, it can be shown that $G_4^0$ has two kinds of poles. It possesses the same poles as the one-electron and one-hole channel of the non-interacting 2-body Green's function and the two-electron and two-hole channel of the non-interacting 4-body Green's function. We define the non-interacting four-particle correlation function $L^0$ as $L^0 = iG_4^0$

$$L^0(\omega) = \begin{pmatrix} L_2^0(\omega) & 0 \\ 0 & L_4^0(\omega) \end{pmatrix} \tag{1}$$

The $L_2^0$ contains poles corresponding to one electron and one hole (two particles) channel, and the $L_4^0$ block contains poles corresponding to two electrons and two holes (four particles) channel of the four-body Green's function. In a single-particle basis, these correlation functions are given by

$$L^0_{2\ p_1p_2,q_1q_2}(\omega) = \frac{\delta_{p_1,q_1}\delta_{p_2,q_2}(f_{p_2}-f_{p_1})}{\omega-(\epsilon_{p_1}-\epsilon_{p_2})+i\Delta sign(f_{p_2}-f_{p_1})} \tag{2}$$

$$\underset{p_1>p_2,\,p_3>p_4,\,q_1>q_2,\,q_3>q_4}{L^0_{4\ p_1p_2p_3p_4,\,q_1q_2q_3q_4}}(\omega) = \frac{\delta_{p_1,q_1}\delta_{p_2,q_2}\delta_{p_3,q_3}\delta_{p_4,q_4}(f_{p_4}-f_{p_1})(f_{p_3}-f_{p_1})(f_{p_4}-f_{p_2})}{\omega-(\epsilon_{p_1}+\epsilon_{p_2}-\epsilon_{p_3}-\epsilon_{p_4})+i\Delta sign(f_{p_4}-f_{p_1})} \tag{3}$$

where $p_n$ and $q_n$ represent states of the one-particle basis set, and they run over the entire basis set without distinguishing between occupied and unoccupied states. $\epsilon_{p_1}$ and $f_{p_1}$ are the energy and occupancy of the $p_1$ state. $\Delta$ represents a positive infinitesimal number ($\Delta \to 0^+$). Since, $L^0_{4\ p_1p_2p_3p_4,q_1q_2q_3q_4}(\omega) = -L^0_{4\ p_2p_1p_3p_4,q_1q_2q_3q_4}(\omega)$, the conditions $p_1 > p_2$ avoid double counting. The MCDE involves Dyson equation of the form

$$L(\omega) = L^0(\omega) + L^0(\omega)\Sigma L(\omega) \tag{4}$$

To leading order in the interactions, the multichannel self-energy $\Sigma$ is frequency independent and is of the form

$$\Sigma = \begin{pmatrix} \Sigma^{2p} & \Sigma^{2p,4p} \\ \Sigma^{4p,2p} & \Sigma^{4p} \end{pmatrix} \tag{5}$$

## IV Recasting the scrCISD Hamiltonian as MCDE

Let $\tilde{L}$ be the four-particle correlation function whose poles correspond to the eigenvalues of the scrCISD Hamiltonian. Then we can write,

$$[\tilde{L}(\omega)]^{-1} = H^{scrCISD} - \omega I \tag{6}$$

The scrCISD Hamiltonian expanded in the combined basis of single and double excitation is given by

$$H^{scrCISD} = \begin{pmatrix} H^{x} & H^{x,xx} \\ H^{xx,x} & H^{xx} \end{pmatrix} \tag{7}$$

The scrCISD Hamiltonian is split into a non-interacting part $\tilde{H}_0$ and an interaction part $\tilde{\Sigma}$.

$$H^{scrCISD} = \tilde{H}_0 + \tilde{\Sigma} \tag{8}$$

$$\tilde{H}_0 = \begin{pmatrix} \tilde{H}^{0,2p} & 0 \\ 0 & \tilde{H}^{0,4p} \end{pmatrix} \tag{9}$$

$$\tilde{\Sigma} = \begin{pmatrix} \tilde{\Sigma}^{2p} & \tilde{\Sigma}^{2p,4p} \\ \tilde{\Sigma}^{4p,2p} & \tilde{\Sigma}^{4p} \end{pmatrix} \tag{10}$$

$$\tilde{H}^{0,2p}_{j\beta,i\alpha} = (\epsilon^{qp}_i - \epsilon^{qp}_\alpha)\,\delta_{ij}\delta_{\alpha\beta} \tag{11}$$

$$\tilde{H}^{0,4p}_{mn\gamma\eta,ij\alpha\beta} = ((\epsilon^{qp}_i + \epsilon^{qp}_j) - (\epsilon^{qp}_\alpha + \epsilon^{qp}_\beta))\delta_{im}\delta_{jn}\delta_{\alpha\gamma}\delta_{\beta\eta} \tag{12}$$

$$\tilde{\Sigma}^{2p}_{j\beta,i\alpha} = +\langle i\beta|\,v\,|\alpha j\rangle - \langle i\beta|\,W\,|j\alpha\rangle \tag{13}$$

$$\begin{aligned}
\tilde{\Sigma}^{4p}_{mn\gamma\eta,ij\alpha\beta} = &+[\langle ij|\,W\,|mn\rangle - \langle ij|\,W\,|nm\rangle]\delta_{\alpha\gamma}\delta_{\eta\beta} \\
&+[\langle\alpha\beta|\,W\,|\gamma\eta\rangle - \langle\alpha\beta|\,W\,|\eta\gamma\rangle]\delta_{mi}\delta_{nj} \\
&-[\langle i\eta|\,v\,|\alpha m\rangle - \langle i\eta|\,W\,|m\alpha\rangle]\,\delta_{jn}\delta_{\beta\gamma} \\
&+[\langle i\eta|\,v\,|\alpha n\rangle - \langle i\eta|\,W\,|n\alpha\rangle]\,\delta_{jm}\delta_{\beta\gamma} \\
&+[\langle j\eta|\,v\,|\alpha m\rangle - \langle j\eta|\,W\,|m\alpha\rangle]\,\delta_{in}\delta_{\beta\gamma} \\
&-[\langle j\eta|\,v\,|\alpha n\rangle - \langle j\eta|\,W\,|n\alpha\rangle]\,\delta_{im}\delta_{\beta\gamma} \\
&-[\langle i\gamma|\,v\,|\beta m\rangle - \langle i\gamma|\,W\,|m\beta\rangle]\,\delta_{jn}\delta_{\alpha\eta} \\
&+[\langle i\gamma|\,v\,|\beta n\rangle - \langle i\gamma|\,W\,|n\beta\rangle]\,\delta_{jm}\delta_{\alpha\eta} \\
&+[\langle j\gamma|\,v\,|\beta m\rangle - \langle j\gamma|\,W\,|m\beta\rangle]\,\delta_{in}\delta_{\alpha\eta} \\
&-[\langle j\gamma|\,v\,|\beta n\rangle - \langle j\gamma|\,W\,|n\beta\rangle]\,\delta_{im}\delta_{\alpha\eta} \\
&+[\langle i\gamma|\,v\,|\alpha m\rangle - \langle i\gamma|\,W\,|m\alpha\rangle]\,\delta_{jn}\delta_{\beta\eta} \\
&-[\langle i\gamma|\,v\,|\alpha n\rangle - \langle i\gamma|\,W\,|n\beta\rangle]\,\delta_{jm}\delta_{\beta\eta} \\
&-[\langle j\gamma|\,v\,|\alpha m\rangle - \langle j\gamma|\,W\,|m\gamma\rangle]\,\delta_{in}\delta_{\beta\eta} \\
&+[\langle j\gamma|\,v\,|\alpha m\rangle - \langle j\gamma|\,W\,|n\alpha\rangle]\,\delta_{im}\delta_{\beta\eta} \\
&+[\langle i\eta|\,v\,|\beta m\rangle - \langle i\eta|\,W\,|m\beta\rangle]\,\delta_{jn}\delta_{\alpha\gamma} \\
&-[\langle i\eta|\,v\,|\beta n\rangle - \langle i\eta|\,W\,|n\beta\rangle]\,\delta_{jm}\delta_{\alpha\gamma} \\
&-[\langle j\eta|\,v\,|\beta m\rangle - \langle j\eta|\,W\,|m\beta\rangle]\,\delta_{in}\delta_{\alpha\gamma} \\
&+[\langle j\eta|\,v\,|\beta n\rangle - \langle j\eta|\,W\,|n\beta\rangle]\,\delta_{im}\delta_{\alpha\gamma}
\end{aligned} \tag{14}$$

$$\begin{aligned}
\tilde{\Sigma}^{2p,4p}_{m\gamma,ij\alpha\beta} = &+[\langle ij|\,W\,|m\alpha\rangle - \langle ij|\,W\,|\alpha m\rangle]\delta_{\beta\gamma} \\
&-[\langle ij|\,W\,|m\beta\rangle - \langle ij|\,W\,|\beta m\rangle]\delta_{\alpha\gamma} \\
&-[\langle\alpha\beta|\,W\,|\gamma i\rangle - \langle\alpha\beta|\,W\,|i\gamma\rangle]\delta_{mj} \\
&+[\langle\alpha\beta|\,W\,|\gamma j\rangle - \langle\alpha\beta|\,W\,|j\gamma\rangle]\delta_{mi}
\end{aligned} \tag{15}$$

$$\tilde{\Sigma}^{4p,2p}_{ij\alpha\beta,m\gamma} = (\tilde{\Sigma}^{2p,4p}_{m\gamma,ij\alpha\beta,})^* \tag{16}$$

Let $\tilde{L^0}$ be the non-interacting four-particle correlation function

$$[\tilde{L}^0(\omega)]^{-1} = \tilde{H}_0 - \omega I \tag{17}$$

$\tilde{L}^0(\omega)$ contains $\tilde{L}^0_2(\omega)$, whose poles correspond to one electron and one hole excitations, and $\tilde{L}^0_4(\omega)$ whose poles correspond to two hole and two electron excitations.

$$\tilde{L}^0(\omega) = \begin{pmatrix} \tilde{L}^0_2(\omega) & 0 \\ 0 & \tilde{L}^0_4(\omega) \end{pmatrix} \tag{18}$$

with,

$$\tilde{L}^0_{j\beta,i\alpha}(\omega) = \frac{\delta_{ij}\delta_{\alpha\beta}}{\omega - (\epsilon^{qp}_i - \epsilon^{qp}_\alpha) + i\Delta} \tag{19}$$

$$\underset{m>n,\,\gamma>\eta,\,i>j,\,\alpha>\beta}{\tilde{L}^0{}_{mn\gamma\eta,ij\alpha\beta}}(\omega) = \frac{\delta_{im}\delta_{jn}\delta_{\alpha\gamma}\delta_{\beta\eta}}{\omega - (\epsilon^{qp}_i + \epsilon^{qp}_j - \epsilon^{qp}_\alpha - \epsilon^{qp}_\beta) + i\Delta} \tag{20}$$

$$[\tilde{L}(\omega)]^{-1} = [\tilde{L}^0(\omega)]^{-1} + \tilde{\Sigma} \tag{21}$$

$$\tilde{L}(\omega) = \tilde{L}^0(\omega) + \tilde{L}^0(\omega)\tilde{\Sigma}\tilde{L}(\omega) \tag{22}$$

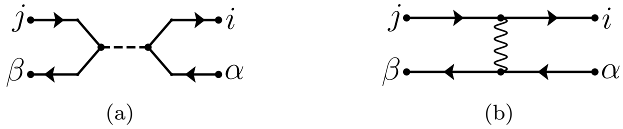


FIG. 1. Two first order diagrams included in $\tilde{L}^{2p}$. Panel (a) corresponds to electron-hole exchange, and panel (b) corresponds to electron-hole direct interaction. The screened Coulomb interaction $W$ is represented by solid wavy lines, and the bare Coulomb interaction is represented by dashed lines.

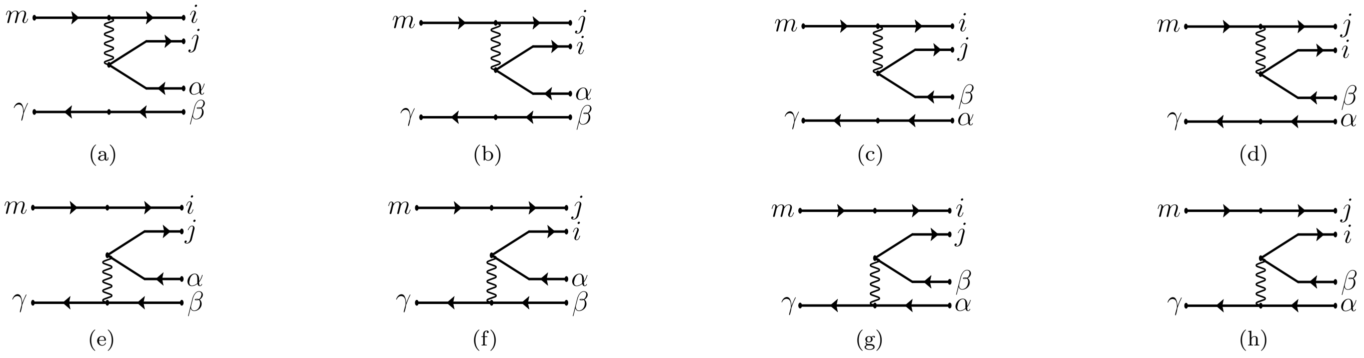


FIG. 2. Eight first order diagrams included in $\tilde{L}^{2p,4p}$

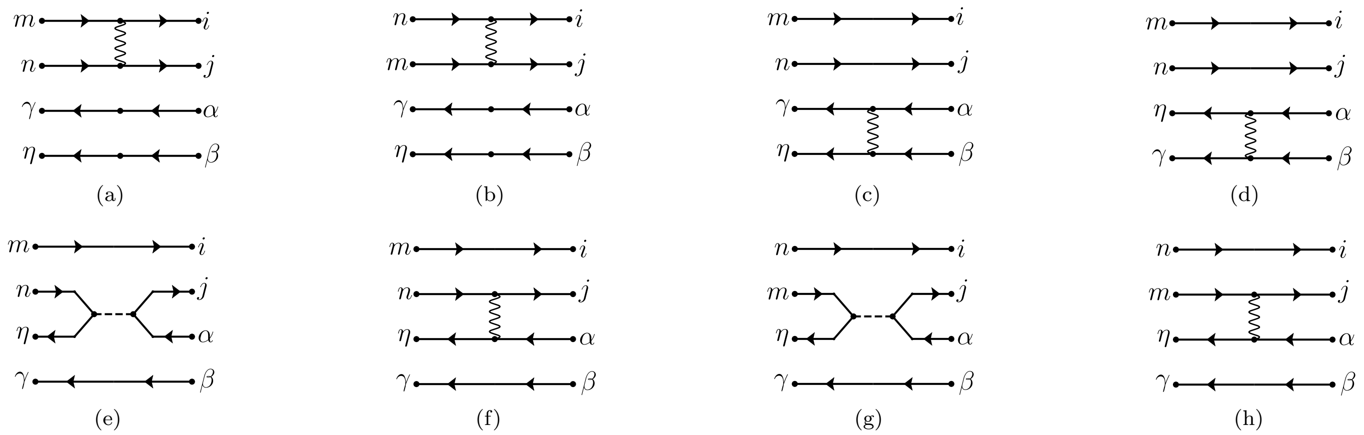


FIG. 3. First-order diagrams included in $\tilde{L}^{4p}$. Panels (a) and (b) show electron–electron interactions, while panels (c) and (d) show hole–hole interactions. Panels (e) and (g) depict electron–hole exchange interactions, and panels (f) and (h) depict electron–hole direct interactions.

# V Differences between MCDE and scrCISD-MCDE

In the scrCISD-MCDE formalism, $\tilde{L}_2^0(\omega)$ contains poles corresponding to single excitations, while $\tilde{L}_4^0(\omega)$ contains poles corresponding to double excitations. In contrast, the MCDE formulation includes poles corresponding to both excitation and de-excitation processes in both the single and double excitation channels—that is, in both $L_2^0(\omega)$ and $L_4^0(\omega)$. The non-interacting two-particle correlation function $L_2^0(t)$ can be written in terms of the one-body time-ordered Green's function $G_1(t)$ as :

$$L_2^0(t) = iG_1(t)G_1(-t) \tag{23}$$

The one-body Green's function can be written as

$$\begin{aligned} G_1(t) &= \theta(t)G_1(t) + \theta(-t)G_1(t) \\ &= \theta(t)G_1^e(t) + \theta(-t)G_1^h(t) \end{aligned} \tag{24}$$

It can be shown that the Fourier transform of $\theta(t)G_1(t)$ contains poles only corresponding to electron states hence represented by $G_1^e(t)$ and the Fourier transform of $\theta(-t)G_1(t)$ contains poles corresponding to hole states hence represented by $G_1^h(t)$.

$$\begin{aligned} L_2^0(t) &= i\theta(t)G_1(t)G_1(-t) + i\theta(-t)G_1(t)G_1(-t) \\ &= i\theta(t)G_1^e(t)G_1^h(-t) + i\theta(-t)G_1^h(t)G_1^e(-t) \end{aligned} \tag{25}$$

It follows that $\theta(t)G_1^e(t)G_1^h(-t)$ contains poles corresponding to single excitations (such at $((\epsilon_i^{qp} - \epsilon_\alpha^{qp}))$, while $\theta(-t)G_1^e(-t)G_1^h(t)$ contains poles corresponding to single de-excitations (such as at $(\epsilon_\alpha^{qp} - \epsilon_i^{qp})$). However, $\tilde{L}_2^0$ of scrCISD-MCDE in time domain can be written as

$$\begin{aligned} \tilde{L}_2^0(t) &= i\theta(t)G_1(t)G_1(-t) \\ &= i\theta(t)G_1^e(t)G_1^h(-t) \end{aligned} \tag{26}$$

Thus $\tilde{L}_2^0$ only contains poles corresponding to excitations. Similarly, $L_4^0(t)$ of MCDE contains both forward and backward time-ordering, thus containing both double excitations and de-excitations in its poles, whereas $\tilde{L}_4^0$ of scrCISD has only forward time ordering thus containing poles only corresponding to double excitations. Since

the propagators in the scrCISD-MCDE contain only one time ordering, the diagrams generated from iterations of scrCISD-MCDE always correspond to a particular time-ordering, in contrast to the Feynman diagrams that include all possible time orderings. Thus, we use Goldstone diagrams rather than Feynman diagrams to represent diagrams within scrCISD-MCDE.

[1] G. D. Scholes, "Correlated pair states formed by singlet fission and exciton–exciton annihilation," The Journal of Physical Chemistry A **119**, 12699–12705 (2015).

[2] M. Schreiber, M. R. Silva-Junior, S. P. A. Sauer, and W. Thiel, "Benchmarks for electronically excited states: CASPT2, CC2, CCSD, and CC3," The Journal of Chemical Physics **128**, 134110 (2008).

[3] F. Bruneval, S. M. Hamed, and J. B. Neaton, "A systematic benchmark of the ab initio Bethe-Salpeter equation approach for low-lying optical excitations of small organic molecules," The Journal of Chemical Physics **142**, 244101 (2015).

[4] G. Riva, P. Romaniello, and J. A. Berger, "Multichannel dyson equation: Coupling many-body green's functions," Phys. Rev. Lett. **131**, 216401 (2023).

[5] G. Riva, P. Romaniello, and J. A. Berger, "Derivation and analysis of the multichannel dyson equation," Phys. Rev. B **110**, 115140 (2024).

[6] G. Riva, T. Fischer, S. Paggi, J. A. Berger, and P. Romaniello, "Multichannel dyson equations for even- and odd-order green's functions: Application to double excitations," Phys. Rev. B **111**, 195133 (2025).
